# Supplementary material for: SparseFormer: Detecting Objects in HRW Shots via Sparse Vision Transformer
Source: arXiv:2502.07216 source file (2025-02-11)
Supplement: Supplementary file 1 [file X_suppl.tex]

\clearpage
\setcounter{page}{1}
\maketitle
% \maketitlesupplementary

This supplementary material contains additional details of the main manuscript. \cref{sec:details} presents additional details of the models and training strategies. 
\cref{sec:CNMS} further explains the \cref{alg:nmbs}. 
\cref{sec:keep} evaluate the reasonableness of the keeping ratio formulation.
% ~\cref{sec:experiment} complements more experiments not included in the main manuscript. 
\cref{sec:viz} shows more visualization results to prove the effectiveness of SparseFormer.
% \cref{sec:dis} provides discussions for people to rethink the paradigm in computer vision. 
\cref{sec:pytorch} provide the PyTorch-like code for SparseFormer.

\section{Details of Models and Training}
\label{sec:details}
\subsection{Dataset Preparation}
\noindent\textbf{PANDA dataset~\cite{wang2020panda} }. PAN~\cite{fan2022speed} prepares the data for training by using a sliding window of 2,048$\times$1,024 pixels to decompose the image which is downsampling with a factor of 4.
In this paper, we use a multi-scale pre-process to accelerate training convergence and boost performance. 
Firstly, we cropped the patches according to a 16$\times$16 grid, an 8$\times$8 grid, and a 4$\times$4 grid on the original image and filter the patch which has no persons.
Then, all of the patches are resized to the same resolution for training.
In other words, our pre-process is using the sliding window on images downsampled at three scales.

\noindent\textbf{DOTA dataset~\cite{xia2018dota}}. We crop the original images into the patches of 1024$\times$1024 with a stride of 824, which means the pixel overlap between two adjacent patches is 200. In our experiment, we do not use multi-scale training and testing and compared with the current state-of-the-art methods which have the same setting.

\begin{figure*}[!]
\centering
	% \begin{center}
		\includegraphics[width=1.0\linewidth]{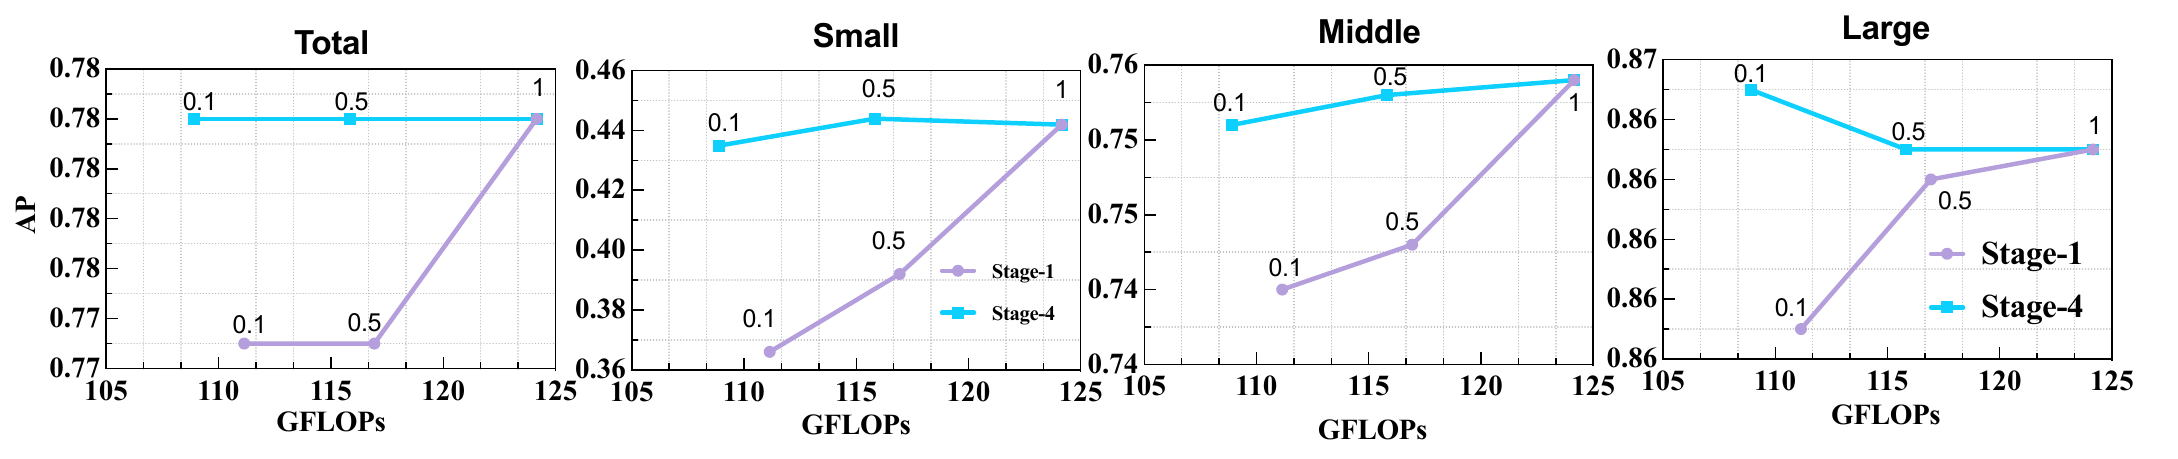}
	% \end{center}
	\caption{Effect of keeping ratio on different stage-1 and stage-4.}
	\label{fig:keeping_ratio}	
\end{figure*}

\subsection{Training and Inference}
The observations in \cite{he2019rethinking} show that training from scratch is no worse than the fine-tuning counterpart.
Thus, we train the detector with 36 epochs instead of pretraining on ImageNet.
This also ensures that we have a fair comparison with Swin Transformer, the performance improvement comes from the novel design rather than better pre-train weight.
Benefiting from the sparse architecture, our model can be easily trained on GeForce RTX 3090Ti GPUs.

During inference,  we divided large-resolution images into patches with a resolution of 6000$\times$3600 and an overlap of 600 pixels between patches for the PANDA dataset, and with a resolution of 1024$\times$1024 and an overlap of 200 pixels between patches for the DOTA dataset.

\section{Algorithm Explanation for C-NMS}
\label{sec:CNMS}
\setlength{\textfloatsep}{5pt}
\begin{algorithm}[t]
\caption {Cross-window NMS (C-NMS)}
\label{alg:nmbs}
% {$\mathcal{B}$ is $N\times4$ matrix of initial detection boxes.
% $\mathcal{S}$ contains corresponding detection scores.
% $\mathcal{C}$ is $N\times4$ matrix of corresponding variances. $\mathcal{D}$ is the final set of detections.
% $\sigma_t$ is a tunable parameter of NMBS. The lines in {\color{blue}blue} and in {\color{ForestGreen}green} are soft-NMS and NMBS\ respectively.}\label{alg:nms}
% \begin{algorithmic}
\SetKwInOut{KwInput}{Variables}
\SetKwInOut{KwOutput}{Functions}
\KwInput{
$\mathcal{B}_{1}$, $\mathcal{B}_{2}$ are candidate box sets from two windows, $\tau$ is the C-NMS threshold\;
}
\KwOutput{
$\mathop{\mathrm{NMS}}(\cdot)$ is the conventional NMS\; \qquad \qquad \quad $\mathop{\mathrm{AREA}}(\cdot)$ calculates the area of a box\;
}
$\mathcal{B}_{1}^{\prime} \gets \mathop{\mathrm{NMS}}(\mathcal{B}_{1}); \mathcal{B}_{2}^{\prime} \gets \mathop{\mathrm{NMS}}(\mathcal{B}_{2})$\;
$\mathcal{B} \gets \mathcal{B}_{1}^{\prime} \cup \mathcal{B}_{2}^{\prime}; \mathcal{B}^{\prime} \gets \emptyset$\;
\While {$\mathcal{B} \ne \emptyset$}{
    $m \gets \mathop{\mathrm{argmax}}_{i} \mathop{\mathrm{AREA}}(b_{i})$, s.t. $b_{i} \in \mathcal{B}$\;
    $ \mathcal{B}^{\prime} \gets \mathcal{B}^{\prime} \cup \left\{b_m \right\}; \mathcal{B} \gets \mathcal{B} - \left\{b_m \right\}$\;
    \For {$b_i \in \mathcal{B}$}{
        \If {$IoU(b_{i}, b_{m}) \ge \tau $}{
            $\mathcal{B} \gets \mathcal{B} - \left\{b_i\right\}$\; 
        }
    }
}
\textbf{return} $\mathcal{B}^{\prime}$\;
\end{algorithm}

Suppose there are only two candidate box sets $\mathcal{B}_{1}$ and $\mathcal{B}_{2}$ for simplicity, indicating the predictions of the object detector on the two overlapped sliding windows. 
We first employ the conventional score-based NMS post-processing on both box sets $\mathcal{B}_{1}$ and $\mathcal{B}_{2}$ to locally eliminate redundant boxes with low confidence. This process results in two locally-suppressed outcomes: $\mathcal{B}_{1}^{\prime}$ and $\mathcal{B}_{2}^{\prime}$. 
Then, for the cross-window box suppression, we unite $\mathcal{B}_{1}^{\prime}$ and $\mathcal{B}_{2}^{\prime}$ to form a union box set $\mathcal{B}$. In order to retain the boxes covering the complete targets, we design to use the area of boxes to suppress boxes located at overlapping regions. 
As in \cref{alg:nmbs}, at each iteration, the box $b_{m}$ with \emph{the largest area} is removed from $\mathcal{B}$ and append to the suppressed set $\mathcal{B}^{\prime}$. We then remove all boxes $b_{i}$ from $\mathcal{B}$, whose IoUs with $b_m$ are greater than a pre-defined threshold $\tau$. The algorithm ends when the box union set $\mathcal{B}$ is empty. This strategy is effective in selecting optimal boxes for HRW shot object detection. 

\begin{figure*}[!]
	\begin{center}
		\includegraphics[width=1.0\linewidth]{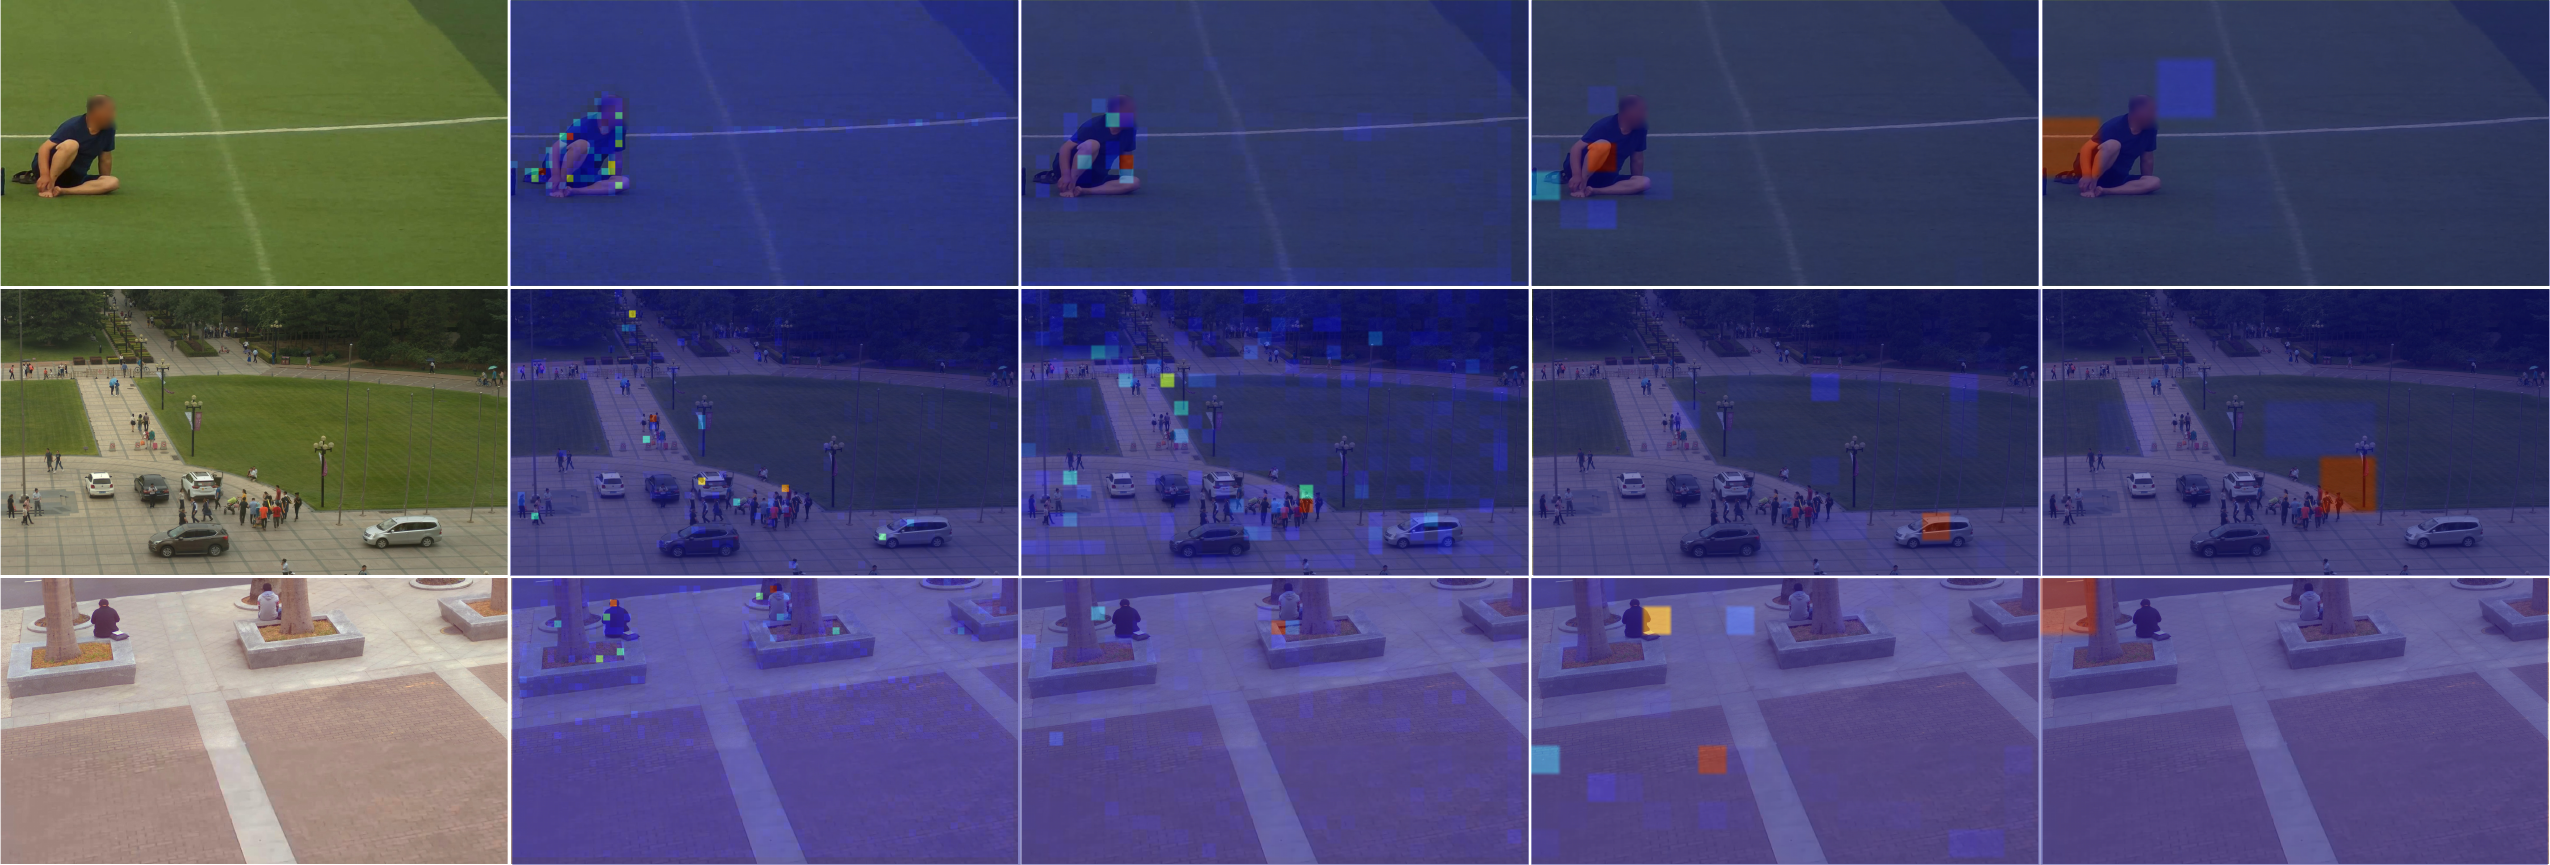}
	\end{center}
	% \vspace{-15pt}
	\caption{\textbf{Visualization of the sparse window scores of four stages.} The samples are from the PNADA dataset~\cite{wang2020panda}. Highlighted patches mean higher scores. It is easy to observe that our model pays more attention to the details of foreground and complex regions.}
	% \vspace{-5pt}
	\label{fig:viz}	
\end{figure*}

% \section{End-to-end Optimization}
% \label{sec:e2e}
% There is an obstacle that the ScoreNet cannot be optimized, since we only use the output to sort the grids and the gradient cannot be back-propagated.
% To address this issue, we use the Gumbel-SoftMax~\cite{maddison2016concrete} trick to relax the sampling process and make it differentiable. It provides a bridge for gradient back-propagation between soft values and binarized values through re-parameterization.
% We also achieve this purpose by re-writing  Equation (5)  to:
% \begin{equation}
%      z \gets  z + (1-s)\times z^{\text{global}}, 
% \label{eq:re_write_update_gloabl}
% \end{equation}
% where $s$ is the output of SoftMax indicating scores of grids.

\begin{table}
\centering
% \vspace{-10pt}
\caption{Ablation studies on sparse ratio.}
% \vspace{-10pt}
\footnotesize
\setlength\tabcolsep{2.2pt}
% \begin{tabularx}{0.48\textwidth}{l|c|*{3}{X}|*{4}{X}}
\begin{tabular}{l|c|*{3}{c}|*{4}{c}}
\hline
\multirow{2}{*}{Method} & \multirow{2}{*}{Ratio} & \multicolumn{3}{c|}{GFLOPs} & \multicolumn{4}{c}{AP}         \\ \cline{3-9} 
                        &                        & Fore   & Back     & All     & Total & Small & Medium & Large \\ \hline
                        & 0.1                & 5.91   & 31.24    & 37.15   & 75.1 & 31.6 & 71.4  & 85.4 \\
                        & 0.3                & 5.90   & 34.14    & 40.04   & 75.9 & 34.5 & 72.7  & 85.3 \\
DyHead                  & 0.5                & 6.16   & 40.59    & 46.75   & 76.5 & 34.7 & 73.5  & 85.5 \\
                        & 0.7                & 6.19   & 60.87    & 67.06   & 77.1 & 36.4 & 74.0  & 86.3 \\
                        & 1.0                & 6.21   & 117.9   & 124.1  & 78.2 & 44.2 & 75.4  & 86.3 \\ \hline
                        & 0.1                & 6.74   & 44.77    & 51.51   & 75.6 & 33.5 & 75.1  & 82.4 \\
                        & 0.3                & 6.79   & 48.86    & 54.65   & 76.1 & 41.1 & 76.2  & 81.3 \\
DINO                    & 0.5                & 6.84   & 52.53    & 59.37   & 76.7 & 42.5 & 77.2  & 80.9 \\
                        & 0.7                & 6.90   & 68.81    & 75.71   & 77.3 & 44.3 & 77.5  & 81.3 \\
                        & 1.0                & 7.06   & 134.2   & 141.3  & 78.0 & 53.0 & 77.8  & 81.9 \\ \hline
\end{tabular}
\label{tab:sparse_ratio}
\end{table}

\section{Study on keeping ratio. } 
\label{sec:keep}
Discarding the worthless grids is an important part of our strategy. So we conduct experiments to study the effect of the keeping ratio of the grids on the final performance.
\cref{tab:sparse_ratio} shows the results and the keeping ratio $k$ is formulated as $[k, k^2, k^3, k^4]$ for each stage.
As the features become more and more sparse, we can see a significant drop in FLOPs but an insignificant drop in accuracy. 
% We further draw a performance curve, which is shown in \cref{fig:sota}.
In order to evaluate the reasonableness of this formulation, 
we conduct experiments on new parameters containing$[k, 1, 1, 1]$ denoted as ``Stage-1'', and $[1, 1, 1, k]$ denoted as ``Stage-4'' with $k \in \{0.1, 0.5, 1\}$.
The results are shown in ~\cref{fig:keeping_ratio}.
From the perspective of the GFLOPs, discarding the tokens in Stage-4 can save more computation than in Stage-1. It is because the most computation of window self-attention is on the MLP layer and the feature in Stage-4 has larger dimensions.
To our surprise, with more sparse windows, Stage-4 can still perform well on total AP.
From the perspective of objects of different scales, more sparse windows~(lower $k$) on Stage-4 can drop the performance on small and middle objects but improve the AP on large objects. The opposite is true for Stage-1. Therefore,
The formulation of $[k, k^2, k^3, k^4]$, with more drop in Stage-4, seems a reasonable choice.

\section{Model Analysis}
\label{sec:viz}
\subsection{Visualization Results}
To further investigate the behavior of the window sparsification, we visualize selected windows of each stage in \cref{fig:viz} to show the advantage of the reduction on the redundancy computation such as background and low-entropy foreground.
The results also demonstrate that our sparse representation learning makes sense and we believe this will become a promising research direction for not only future detection but any other vision tasks.
% In this section, we provide more visualization results to show the effectiveness of SparseFormer. 
The selected windows of each stage on the DOTA dataset are shown in \cref{fig:DOTA}.
The results show that when there is more background and less foreground, our local self-attention is more concentrated in the foreground region. When it is all background, the scores are relatively even across all regions.
To our surprise, Stage-2 usually generates a more even score map which might show its importance among the four stages.
This is also an important basis for further exploring how to design more efficient sparse architecture.

\begin{figure*}[!]
	\begin{center}
		\includegraphics[width=1.0\linewidth]{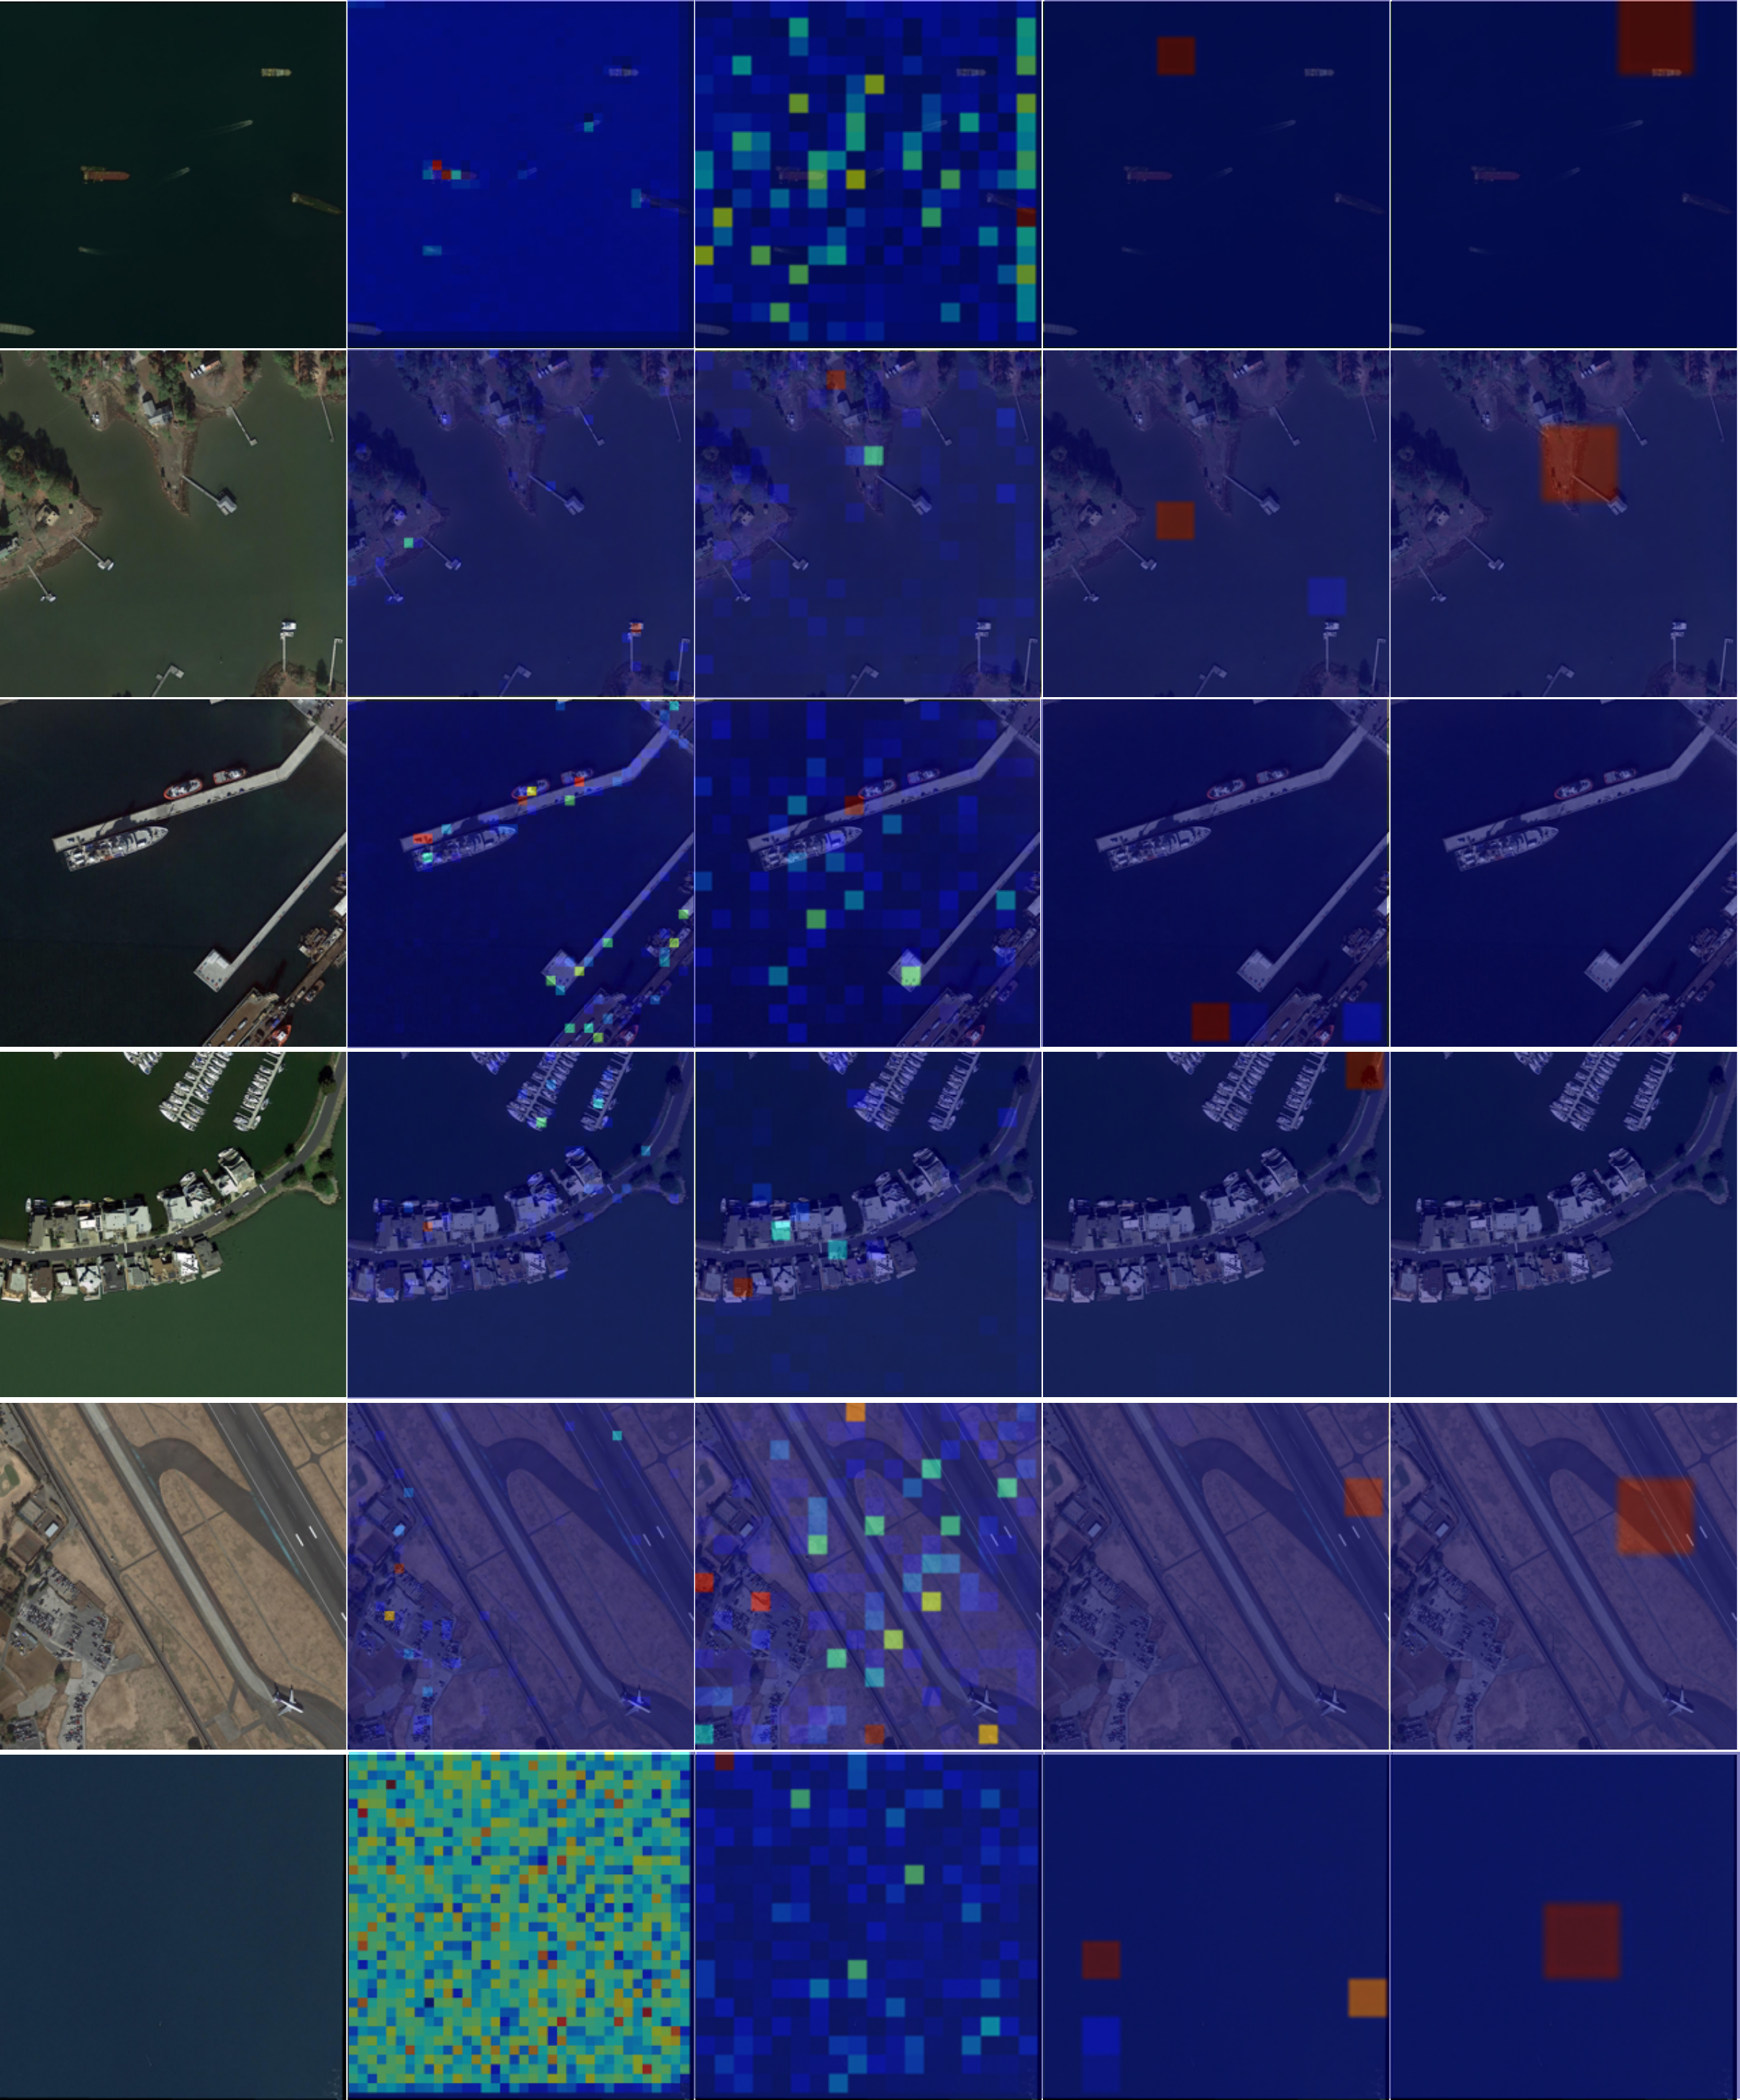}
	\end{center}
	% \vspace{-10pt}
	\caption{\textbf{Visualization of the sparse window scores of each stage on DOTA dataset.}The samples are from the DOTA dataset~\cite{xia2018dota}.}
	% \vspace{-15pt}
	\label{fig:DOTA}	
\end{figure*}

\begin{figure*}[!]
	\begin{center}
		\includegraphics[width=1.0\linewidth]{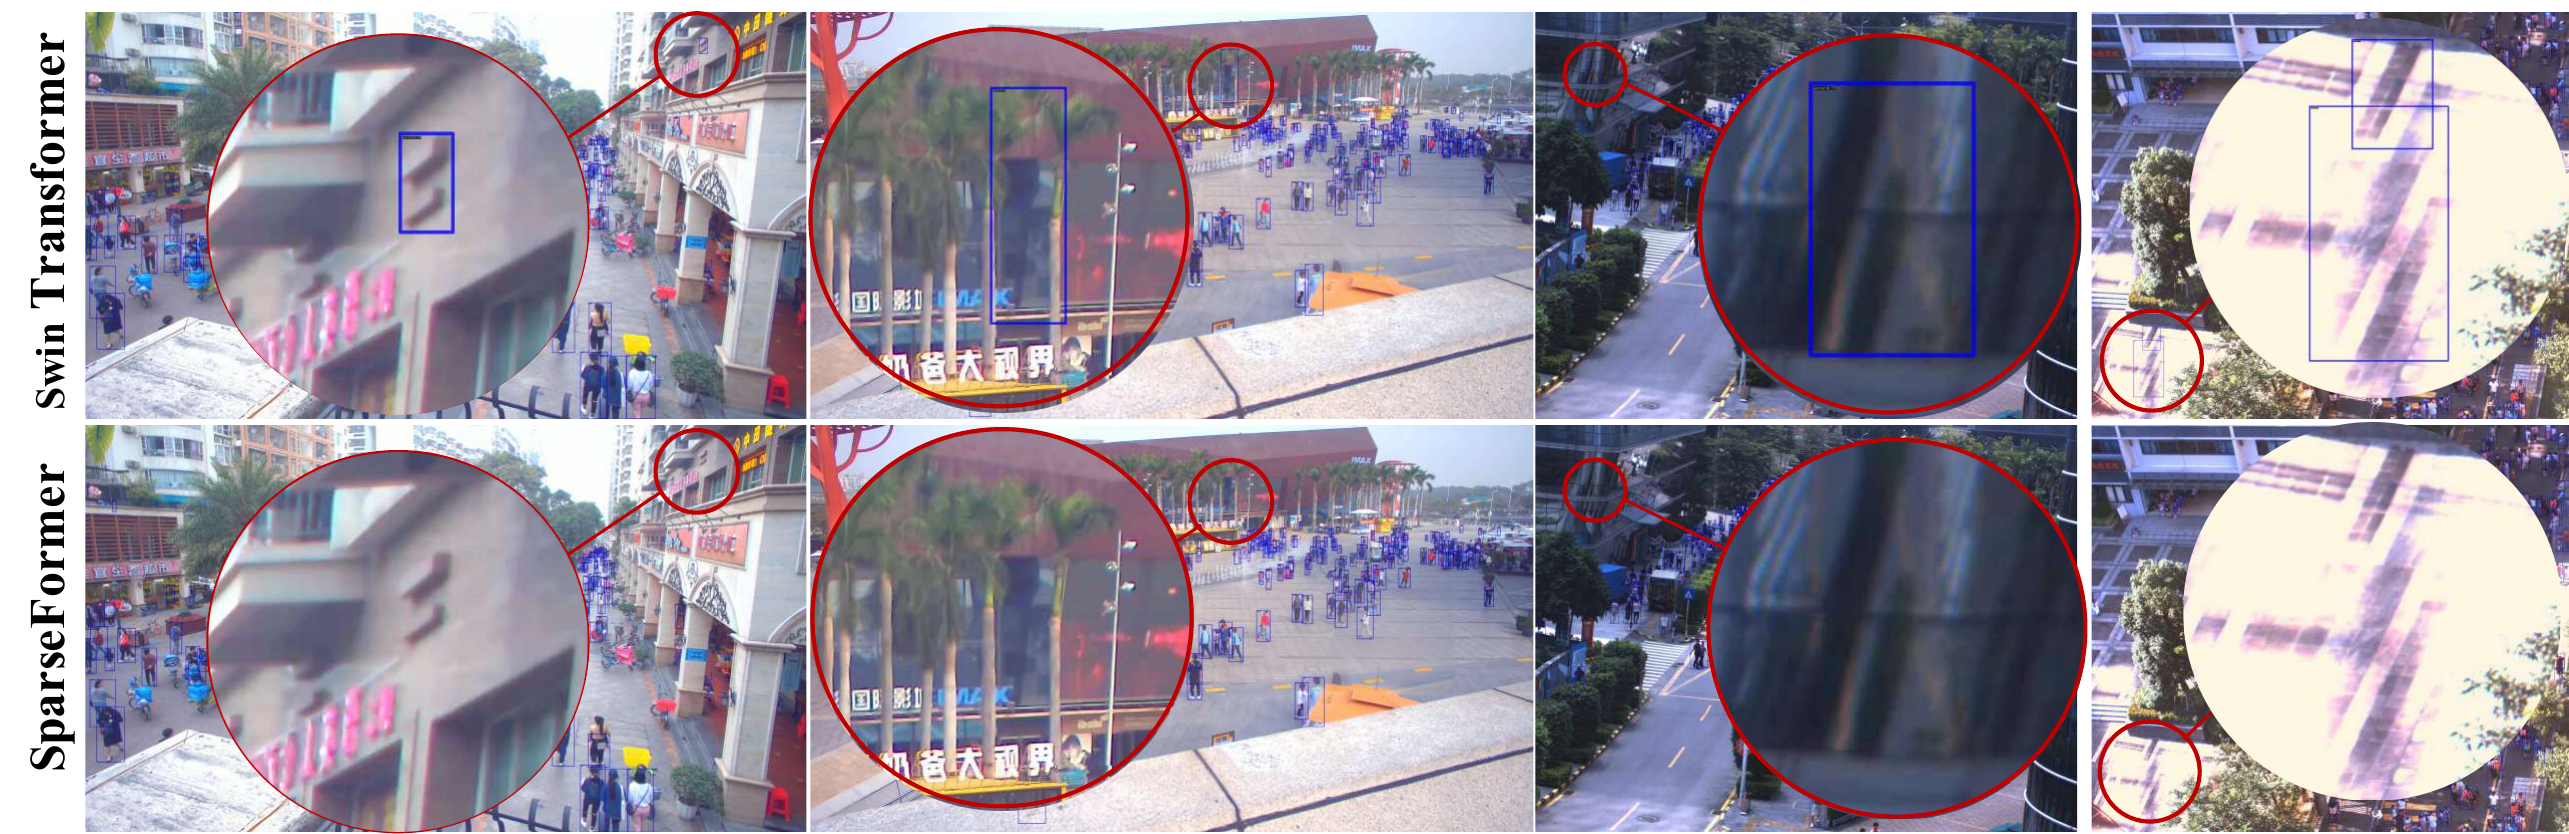}
	\end{center}
	% \vspace{-15pt}
	\caption{\textbf{Qualitative results.} We compare our SparseFormer to the Swin TransFormer and  our model has fewer false positives thanks to a sparse sampling of the background.}
	% \vspace{-15pt}
	\label{fig:fp}	
\end{figure*}

\subsection{Qualitative comparison of detection results.} 
We present qualitative results in ~\cref{fig:fp}
to compare the SparseFormer and Swin Transformer.
We observe that through the token sparsification on the background, SparseFormer has lower false positive examples.

\section{Code in PyTorch}
\label{sec:pytorch}
The local block is an essential module for reducing the computation, and it can be easily implemented by inserting a plug-in module into the original network.
We provide the PyTorch-like pseudocode in \cref{alg:att} and \cref{alg:ffn} associated with the Local self-attention block. \cref{alg:block}
further shows the SparseFormer block built with these modules.
It can be seen from the pseudocode that our sparse design is not limited to the Transformer but also could modify the convolution neural network like ResNet~\cite{he2016deep} by adding windows.
The whole code will be publicly released after the review process.

\begin{algorithm*}[t]
\caption{Sparse Window based Multi-head Self-attention, PyTorch-like Pseudocode}
\label{alg:att}
\definecolor{codeblue}{rgb}{0.25,0.5,0.5}
\definecolor{codekw}{rgb}{0.85, 0.18, 0.50}
\lstset{
  backgroundcolor=\color{white},
  basicstyle=\fontsize{7.5pt}{7.5pt}\ttfamily\selectfont,
  columns=fullflexible,
  breaklines=true,
  captionpos=b,
  commentstyle=\fontsize{7.5pt}{7.5pt}\color{codeblue},
  keywordstyle=\fontsize{7.5pt}{7.5pt}\color{codekw},
}
\begin{lstlisting}[language=python]

class SparseWindowMSA(BaseModule):

    def forward(self, query, hw_shape, keep_token_indices):
        B, L, C = query.shape
        H, W = hw_shape
        K = keep_token_indices.shape[1]
        query = query.view(B, H, W, C)

        # pad feature maps to multiples of window size
        pad_r = (self.window_size - W % self.window_size) % self.window_size
        pad_b = (self.window_size - H % self.window_size) % self.window_size
        query = F.pad(query, (0, 0, 0, pad_r, 0, pad_b))
        H_pad, W_pad = query.shape[1], query.shape[2]

        # cyclic shift 
        shifted_query = shift_function(query)

        # B, nW, window_size, window_size, C
        query_windows = self.window_partition(shifted_query)

        # ********************************************plug-in********************************************
        # sparse windows:nW->K (B, K, window_size, window_size, C)
        query_windows_sparse = torch.gather(query_windows, sparse_grad=True, dim=1, index=keep_token_indices)
        query_windows_sparse = query_windows_sparse.view(-1, self.window_size**2, C)
        # ***********************************************************************************************

        # W-MSA/SW-MSA (B*K, window_size*window_size, C)
        attn_windows_sparse = self.w_msa(query_windows_sparse, mask=attn_mask_sparse)
        
        # ********************************************plug-in********************************************
        # (B, K, window_size, window_size, C)
        attn_windows_sparse = attn_windows_sparse.view(B, -1, self.window_size, self.window_size, C)
        # inverse sparse:K->nW (B, nW, window_size, window_size, C)
        attn_windows = query_windows.scatter(src=attn_windows_sparse, dim=1, index=keep_token_indices)
        # ***********************************************************************************************
        
        # (B, H_pad, W_pad, C)
        shifted_x = self.window_reverse(attn_windows, H_pad, W_pad)

        # reverse cyclic shift
        x = shift_function(shifted_x)

        if pad_r > 0 or pad_b:
            x = x[:, :H, :W, :].contiguous()
        x = x.view(B, H * W, C)
        x = self.drop(x)
        return x
\end{lstlisting}
\end{algorithm*}

% %%%%%%%%% Algorithm: sparse window
% \begin{algorithm*}[t]
% \caption{Sparse window based multi-head self-attention, PyTorch-like Code}
% \label{alg:att}
% \definecolor{codeblue}{rgb}{0.25,0.5,0.5}
% \definecolor{codekw}{rgb}{0.85, 0.18, 0.50}
% \lstset{
%   backgroundcolor=\color{white},
%   basicstyle=\fontsize{7.5pt}{7.5pt}\ttfamily\selectfont,
%   columns=fullflexible,
%   breaklines=true,
%   captionpos=b,
%   commentstyle=\fontsize{7.5pt}{7.5pt}\color{codeblue},
%   keywordstyle=\fontsize{7.5pt}{7.5pt}\color{codekw},
% }
% \begin{lstlisting}[language=python]
% from module import WindowMSA, BaseModule

% class LocalWindowMSA(BaseModule):

%     def __init__(self,
%                  embed_dims,
%                  num_heads,
%                  window_size,
%                  shift_size=0,
%                  qkv_bias=True,
%                  qk_scale=None,
%                  attn_drop_rate=0,
%                  proj_drop_rate=0,
%                  dropout_layer=dict(type='DropPath', drop_prob=0.),
%                  init_cfg=None):
%         super().__init__(init_cfg)

%         self.window_size = window_size
%         self.shift_size = shift_size

%         self.w_msa = WindowMSA(
%             embed_dims=embed_dims,
%             num_heads=num_heads,
%             window_size=to_2tuple(window_size),
%             qkv_bias=qkv_bias,
%             qk_scale=qk_scale,
%             attn_drop_rate=attn_drop_rate,
%             proj_drop_rate=proj_drop_rate,
%             init_cfg=None)

%         self.drop = build_dropout(dropout_layer)

%     def forward(self, query, hw_shape, keep_token_indices):
%         B, L, C = query.shape
%         H, W = hw_shape
%         K = keep_token_indices.shape[1]
%         query = query.view(B, H, W, C)

%         # pad feature maps to multiples of window size
%         pad_r = (self.window_size - W % self.window_size) % self.window_size
%         pad_b = (self.window_size - H % self.window_size) % self.window_size
%         query = F.pad(query, (0, 0, 0, pad_r, 0, pad_b))
%         H_pad, W_pad = query.shape[1], query.shape[2]

%         # cyclic shift (This part is the same as Swin Transformer so it is not shown here).
%         shifted_query = query

%         query_windows = self.window_partition(shifted_query)
%         query_windows = query_windows.view(B, -1, self.window_size, self.window_size, C)

%         if attn_mask is not None:
%             attn_mask_sparse = torch.gather(attn_mask, sparse_grad=True, dim=1,
%                                      index=keep_token_indices.view(B, K, 1, 1).repeat(1, 1, self.window_size**2,
%                                                                                          self.window_size**2))
%             attn_mask_sparse =  attn_mask_sparse.view(-1, self.window_size**2, self.window_size**2)
%         else:
%             attn_mask_sparse = None

%         query_windows_sparse = torch.gather(query_windows, sparse_grad=True, dim=1,
%                                             index=keep_token_indices.view(B, K, 1, 1, 1).repeat(1, 1, self.window_size,
%                                                                                           self.window_size, C))
%         query_windows_sparse = query_windows_sparse.view(-1, self.window_size**2, C)

%         attn_windows = self.w_msa(query_windows_sparse, mask=attn_mask_sparse)

%         attn_windows = attn_windows.view(B, -1, self.window_size, self.window_size, C)
%         attn_windows = query_windows.scatter(src=attn_windows, dim=1,
%                                      index=keep_token_indices.view(B, K, 1, 1, 1).repeat(1, 1, self.window_size,
%                                                                                          self.window_size, C))
%         attn_windows = attn_windows.view(-1, self.window_size,
%                                          self.window_size, C)
%         shifted_x = self.window_reverse(attn_windows, H_pad, W_pad)

%         # reverse cyclic shift (not show)
%         x = shifted_x

%         if pad_r > 0 or pad_b:
%             x = x[:, :H, :W, :].contiguous()
%         x = x.view(B, H * W, C)
%         x = self.drop(x)
%         return x
% \end{lstlisting}
% \end{algorithm*}

%%%%%%%%% Algorithm: modules
\begin{algorithm*}[t]
\caption{Sparse Feed-forward Network, PyTorch-like Pseudocode}
\label{alg:ffn}
\definecolor{codeblue}{rgb}{0.25,0.5,0.5}
\definecolor{codekw}{rgb}{0.85, 0.18, 0.50}
\lstset{
  backgroundcolor=\color{white},
  basicstyle=\fontsize{7.5pt}{7.5pt}\ttfamily\selectfont,
  columns=fullflexible,
  breaklines=true,
  captionpos=b,
  commentstyle=\fontsize{7.5pt}{7.5pt}\color{codeblue},
  keywordstyle=\fontsize{7.5pt}{7.5pt}\color{codekw},
}
\begin{lstlisting}[language=python]
from module import FFN, BaseModule

class SparseFFN(BaseModule):

    def forward(self, x, hw_shape, keep_token_indices, identity):

        B, L, C = x.shape
        H, W = hw_shape
        K = keep_token_indices.shape[1]
        query = x.view(B, H, W, C)

        # pad feature maps to multiples of window size
        pad_r = (self.window_size - W % self.window_size) % self.window_size
        pad_b = (self.window_size - H % self.window_size) % self.window_size
        query = F.pad(query, (0, 0, 0, pad_r, 0, pad_b))
        H_pad = query.shape[1]
        W_pad = query.shape[2]

        # B, nW, window_size, window_size, 
        query_windows = self.window_partition(query)
        
        # ********************************************plug-in********************************************
        # sparse windows:nW->K (B, K, window_size, window_size, C
        query_windows_sparse = torch.gather(query_windows, sparse_grad=True, dim=1, index=keep_token_indices)
        # ***********************************************************************************************

        output = self.ffn(query_windows_sparse)


        # ********************************************plug-in********************************************
        # inverse sparse:K->nW (B, nW, window_size, window_size, C)
        x = query_windows.scatter(src=output, dim=1, index=keep_token_indices)
        # ***********************************************************************************************  
        
        # merge windows
        x = x.view(-1, self.window_size, self.window_size, C)
        x = self.window_reverse(x, H_pad, W_pad)
        if pad_r > 0 or pad_b:
            x = x[:, :H, :W, :].contiguous()
        x = x.view(B, H * W, C)

        if not self.add_identity:
            return x
        return x + identity
\end{lstlisting}
\end{algorithm*}

% %%%%%%%%% Algorithm: modules
% \begin{algorithm*}[t]
% \caption{Sparse feed-forward network, PyTorch-like Code}
% \label{alg:ffn}
% \definecolor{codeblue}{rgb}{0.25,0.5,0.5}
% \definecolor{codekw}{rgb}{0.85, 0.18, 0.50}
% \lstset{
%   backgroundcolor=\color{white},
%   basicstyle=\fontsize{7.5pt}{7.5pt}\ttfamily\selectfont,
%   columns=fullflexible,
%   breaklines=true,
%   captionpos=b,
%   commentstyle=\fontsize{7.5pt}{7.5pt}\color{codeblue},
%   keywordstyle=\fontsize{7.5pt}{7.5pt}\color{codekw},
% }
% \begin{lstlisting}[language=python]
% from module import FFN, BaseModule

% class SparseFFN(BaseModule):
%     def __init__(self,
%                  embed_dims=256,
%                  feedforward_channels=1024,
%                  num_fcs=2,
%                  act_cfg=dict(type='ReLU', inplace=True),
%                  drop_rate=0.,
%                  drop_path_rate=0.,
%                  add_identity=True,
%                  init_cfg=None,
%                  **kwargs):
%         super().__init__(init_cfg)
%         self.add_identity = add_identity
%         self.ffn = FFN(
%             embed_dims=embed_dims,
%             feedforward_channels=feedforward_channels,
%             num_fcs=num_fcs,
%             ffn_drop=drop_rate,
%             dropout_layer=dict(type='DropPath', drop_prob=drop_path_rate),
%             act_cfg=act_cfg,
%             add_identity=False,
%             init_cfg=None)

%     def forward(self, x, hw_shape, keep_token_indices, identity):

%         B, L, C = x.shape
%         H, W = hw_shape
%         K = keep_token_indices.shape[1]
%         query = x.view(B, H, W, C)

%         # pad feature maps to multiples of window size
%         pad_r = (self.window_size - W % self.window_size) % self.window_size
%         pad_b = (self.window_size - H % self.window_size) % self.window_size
%         query = F.pad(query, (0, 0, 0, pad_r, 0, pad_b))
%         H_pad = query.shape[1]
%         W_pad = query.shape[2]

%         query_windows = self.window_partition(query)
%         query_windows = query_windows.view(B, -1, self.window_size, self.window_size, C)
%         query_windows_sparse = torch.gather(query_windows, sparse_grad=True, dim=1,
%                                             index=keep_token_indices.view(B, K, 1, 1, 1).repeat(1, 1,
%                                                                                                 self.window_size,
%                                                                                                 self.window_size,
%                                                                                                 C))

%         output = self.ffn(query_windows_sparse)


%         output = output.view(B, -1, self.window_size, self.window_size, C)
%         x = query_windows.scatter(src=output, dim=1,
%                                              index=keep_token_indices.view(B, K, 1, 1, 1).repeat(1, 1,
%                                                                                                  self.window_size,
%                                                                                                  self.window_size,
%                                                                                                  C))
%         # merge windows
%         x = x.view(-1, self.window_size, self.window_size, C)
%         x = self.window_reverse(x, H_pad, W_pad)
%         if pad_r > 0 or pad_b:
%             x = x[:, :H, :W, :].contiguous()
%         x = x.view(B, H * W, C)

%         if not self.add_identity:
%             return x
%         return x + identity
% \end{lstlisting}
% \end{algorithm*}

%%%%%%%%% Algorithm: block

\begin{algorithm*}[t]
\caption{Local Self-attention Block, PyTorch-like Pseudocode}
\label{alg:block}
\definecolor{codeblue}{rgb}{0.25,0.5,0.5}
\definecolor{codekw}{rgb}{0.85, 0.18, 0.50}
\lstset{
  backgroundcolor=\color{white},
  basicstyle=\fontsize{7.5pt}{7.5pt}\ttfamily\selectfont,
  columns=fullflexible,
  breaklines=true,
  captionpos=b,
  commentstyle=\fontsize{7.5pt}{7.5pt}\color{codeblue},
  keywordstyle=\fontsize{7.5pt}{7.5pt}\color{codekw},
}
\begin{lstlisting}[language=python]

class LocalBlock(BaseModule):
    def __init__(self,
                 embed_dims,
                 num_heads,
                 feedforward_channels,
                 window_size=7,
                 shift=False,
                 qkv_bias=True,
                 qk_scale=None,
                 drop_rate=0.,
                 attn_drop_rate=0.,
                 drop_path_rate=0.,
                 act_cfg=dict(type='GELU'),
                 norm_cfg=dict(type='LN'),
                 init_cfg=None):

        super(LocalBlock, self).__init__()

        self.init_cfg = init_cfg
        self.with_cp = with_cp
        self.window_size = window_size

        self.norm1 = build_norm_layer(norm_cfg, embed_dims)[1]
        self.attn = SparseWindowMSA(
            embed_dims=embed_dims,
            num_heads=num_heads,
            window_size=window_size,
            shift_size=window_size // 2 if shift else 0,
            qkv_bias=qkv_bias,
            qk_scale=qk_scale,
            attn_drop_rate=attn_drop_rate,
            proj_drop_rate=drop_rate,
            dropout_layer=dict(type='DropPath', drop_prob=drop_path_rate),
            init_cfg=None)

        self.norm2 = build_norm_layer(norm_cfg, embed_dims)[1]
        self.ffn = SparseFFN(
            embed_dims=embed_dims,
            feedforward_channels=feedforward_channels,
            num_fcs=2,
            ffn_drop=drop_rate,
            dropout_layer=dict(type='DropPath', drop_prob=drop_path_rate),
            act_cfg=act_cfg,
            add_identity=False,
            init_cfg=None)
            
            
    def forward(self, x, hw_shape, keep_token_indices):
        identity = x
        x = self.norm1(x)
        x = self.attn(x, hw_shape, keep_token_indices)

        x = x + identity

        identity = x
        x = self.norm2(x)
        x = self.ffn(x, hw_shape, keep_token_indices, identity=identity)

        return x
            
\end{lstlisting}
\end{algorithm*}
